# Supplementary material for: Adiabatic passage to the continuum
Source: arXiv:1807.01465 ancillary file (2018-07-04)
Supplement: Supplementary file 1 [file capic-suppl.pdf]

# Supplement "Adiabatic passage to the continuum"

Ulf Saalmann, Sajal Kumar Giri, and Jan M. Rost

Technical details for laser pulses and the treatment of the time-dependent Schrödinger equation, with all of them being standard, are provided. Parameters for the numerical calculations are specified. Furthermore, we give details for deriving the conditions for ionization suppression. Finally, a proof for pulses "flipped" in time is given.

## 1 Chirped laser pulses

We consider only Gaussian pulses

$$\mathcal{A}_\beta(t) = \mathcal{A}_\beta\, g_\beta(t) \cos\big(\phi_\beta(t)\big) \quad \text{with the envelope} \quad g_\beta(t) = \mathrm{e}^{-2\ln 2\, t^2/T_\beta{}^2}, \tag{S1a}$$

$\mathcal{A}_\beta$ being the peak value of the vector potential and $T_\beta$ the full-width-at-half-maximum pulse duration. By means of a quadratic modification of the phase in the frequency domain around the central frequency $\omega_0$

$$\widetilde{\phi}_\beta(\omega) = \beta \frac{T^2}{4\ln 2}[\omega - \omega_0]^2, \tag{S1b}$$

the phase in time in Eq. (S1a) grows also quadratically [1]

$$\phi_\beta(t) = \omega_0 t + \frac{\chi_\beta}{2}\frac{t^2}{T^2} \quad \text{with the pre-factor} \quad \chi_\beta \equiv \frac{4\ln 2}{\beta + 1/\beta}. \tag{S1c}$$

This results in a linear chirp of the instantaneous frequency $\omega_\beta(t) = \frac{\mathrm{d}}{\mathrm{d}t}\phi_\beta(t)$

$$\omega_\beta(t) = \omega_0 + \chi_\beta \frac{t}{T^2}. \tag{S1d}$$

The rate of frequency change is $\frac{\mathrm{d}}{\mathrm{d}t}\omega_\beta(t) = \chi_\beta/T^2$, which becomes largest for a given pulse duration $T$ where the prefactor $\chi_\beta$ is maximal. This occurs for $\beta = \pm 1$, with $\frac{\mathrm{d}}{\mathrm{d}t}\omega_{\beta=\pm 1} = \pm 2\ln 2/T^2$. Note that a finite chirp $\beta$ modifies the effective strength and pulse duration in the envelope function (S1a) according to

$$\mathcal{A}_\beta = \frac{\mathcal{A}_{\max}}{\sqrt[4]{1+\beta^2}} \quad \text{and} \quad T_\beta = \sqrt{1+\beta^2}\, T. \tag{S1e}$$

Thus, chirped pulses are longer and weaker, but the product $\mathcal{A}_\beta{}^2 T_\beta$ is constant, i. e., the energy of the pulse does not depend on the chirp $\beta$. This is just a manifestation of Parseval's theorem: Since we do not change the absolute value in the frequency domain, but just the phase as in Eq. (S1b), the integral of the absolute square in the time domain is also unchanged.

Throughout the text we will use the dimension-less quantity $\beta$ in order to characterize the chirp of the pulse.

## 2 Time-dependent Schrödinger equation

### 2.1 Basis-set representation

We will discuss the time evolution of the electron state $\psi(t)$ due to the Hamiltonian $\hat{H}(t) = \hat{H}_0 + \mathcal{A}_\beta(t)\,\hat{p}$ in terms of a field-free basis $\hat{H}_0\varphi_j = E_j\varphi_j$. For

$$\psi(t) = \sum_j \mathrm{e}^{\mathrm{i}\chi_j}\varphi_j a_j(t) \quad \text{and} \quad V_{jj'} = \mathrm{e}^{-\mathrm{i}[\chi_j - \chi_{j'}]}\langle\varphi_j|\hat{p}|\varphi_{j'}\rangle. \tag{S2}$$

the time-dependent Schrödinger equation (TDSE) reads

$$\mathrm{i}\,\dot{a}_j(t) = \sum_{j'} \left[E_j\delta_{jj'} + \mathcal{A}_\beta(t)\,V_{jj'}\right] a_{j'}(t). \tag{S3}$$

This description applies for both cases discussed in the text, the 1D model system and the 3D case of helium. The additional phase factors in the expansion (S2) allow for working with real Hamilton matrices. We chose $\chi_j = (-1)^j\pi/4$ and $\chi_j = (-1)^{\ell_j}\pi/4$ for the 1D and 3D case, respectively. In the 1D case $j$ is odd/even for a gerade/ungerade state $\varphi_j$, in the 3D case $\ell_j$ is the angular momentum of the field-free state $\varphi_j$.

### 2.2 Two-level system and rapid adiabatic passage

For a two-level system we use

$$c_0(t) \equiv \mathrm{e}^{\mathrm{i}[E_0t-\phi_\beta(t)+E_1t]/2}a_0(t),\; c_1(t) \equiv \mathrm{e}^{\mathrm{i}[E_0t+\phi_\beta(t)+E_1t]/2}a_1(t) \tag{S4}$$

to get instead of (S3)

$$\mathrm{i}\begin{pmatrix}\dot{c}_0(t)\\ \dot{c}_1(t)\end{pmatrix} = \begin{pmatrix}+\frac{1}{2}\Delta_\beta(t) & \frac{1}{2}\Omega_{01}(t)\\ \frac{1}{2}\Omega_{10}(t) & -\frac{1}{2}\Delta_\beta(t)\end{pmatrix}\begin{pmatrix}c_0(t)\\ c_1(t)\end{pmatrix}, \tag{S5}$$

with the Rabi frequency and the detuning

$$\Omega_{jj'}(t) \equiv g_\beta(t)\,V_{jj'}, \qquad \Delta_\beta(t) = E_0+\omega_\beta(t) - E_1. \tag{S6}$$

Hereby we have used the time-dependent frequency (S1d) and simplified the coupling by means of the rotating-wave approximation, i. e. replaced $\cos\big(\phi(t)\big)$ by either $\frac{1}{2}\mathrm{e}^{+\mathrm{i}\phi(t)}$ or $\frac{1}{2}\mathrm{e}^{-\mathrm{i}\phi(t)}$.

The TDSE (S5) describes the process of rapid adiabatic passage [2]. Hereby one transfer the population from one state to the other by adiabatically changing the character of eigenstate including the non-diagonal coupling terms.

### 2.3 Dressed-state description

Similar to Eq. (S4) one can split the amplitudes $a_j(t)$ into a sum as

$$a_j(t) = \sum_k c_{jk}(t)\mathrm{e}^{\mathrm{i}k\phi_\beta(t)}, \tag{S7}$$

which results in a partitioned TDSE

$$\mathrm{i}\,\dot{c}_{jk}(t) = \left[E_j + k\,\omega_\beta(t)\right] c_{jk}(t) + \sum_{k'=k\pm1}\sum_{j'} \Omega_{jj'}(t)\,c_{j'k'}(t) \tag{S8a}$$

$$\text{with} \quad \Omega_{jj'}(t) \equiv \frac{\mathcal{A}_\beta}{2} g_\beta(t)\,V_{jj'}. \tag{S8b}$$

In principle the sum over $k$ runs from $-\infty$ to $+\infty$, but one can limit it to finite values. The coupling matrix $\Omega_{jj'}$ is proportional to the envelope $g_\beta$ of the pulse (S1), the oscillations are transferred to the diagonal blocks. It has only finite values for states that are coupled: For the 1D model discussed in the text this requires that (i) one of states is gerade and the other one is ungerade and (ii) the "photon-number" difference should be $|k-k'| = 1$.

### 2.3 Numerical propagation

The TDSEs for both, the 1D model system and the 3D helium atom, are propagated in terms of field-free eigenstates. Therefore, eigenenergies and eigenfunctions as well the corresponding

dipole matrix elements are calculated numerically. For the 1D model we considered the lowest 200 states in a box of size $x = -250\,\mathrm{a}_0 \ldots +250\,\mathrm{a}_0$ (with $\mathrm{a}_0$ being the Bohr radius) and used a Numerov approach with a step size of $\delta x = 0.1\,\mathrm{a}_0$. For the 3D helium atom we use an effective potential [3]. For angular momenta $\ell = 0 \ldots 4$ we calculated the lowest 750 states in a box of size $r = 0 \ldots 10^3\mathrm{a}_0$ with a Numerov step size of $\delta r = 0.01\,\mathrm{a}_0$. For the longer pulses shown in Fig. 5 of the main text we used 2250 states with $r_{\max} = 3{\times}10^3\,\mathrm{a}_0$ (for $T > 4\,\mathrm{fs}$) and 3750 states with $r_{\max} = 5{\times}10^3\,\mathrm{a}_0$ (for $T > 12\,\mathrm{fs}$), respectively.

## 3 Suppression of ionization

### 3.1 Dressed-state description

In order to understand the ionization dynamics it is sufficient to consider a set of essential states, which consist of the ground state ($E_0$), the excited state ($E_1$), and a gerade ($E_\mathrm{g}$) and an ungerade ($E_\mathrm{u}$) continuum state, respectively. Those states, in its original and dressed form, build this effective Hamilton matrix

$$H_\mathrm{eff}(t) = \left(\begin{array}{c|ccc|cc|cc}
\overline{E}_0+2\omega & \Omega_{01} & 0 & 0 & 0 & 0 & 0 & \Omega_{0\mathrm{u}} \\ \hline
\Omega_{10} & \widetilde{E}_1+\omega & 0 & 0 & \Omega_{1\mathrm{g}} & 0 & 0 & 0 \\
0 & 0 & \overline{E}_\mathrm{g}+\omega & 0 & 0 & \Omega_\mathrm{gu} & 0 & 0 \\
0 & 0 & 0 & \widetilde{E}_\mathrm{u}+\omega & \Omega_\mathrm{ug} & 0 & 0 & 0 \\ \hline
0 & \Omega_{\mathrm{g}1} & 0 & \Omega_\mathrm{gu} & \overline{E}_\mathrm{g} & 0 & 0 & \Omega_\mathrm{gu} \\
0 & 0 & \Omega_\mathrm{ug} & 0 & 0 & \widetilde{E}_\mathrm{u} & \Omega_\mathrm{ug} & 0 \\ \hline
0 & 0 & 0 & 0 & 0 & \Omega_\mathrm{gu} & \overline{E}_\mathrm{g}-\omega & 0 \\
\Omega_{\mathrm{u}0} & 0 & 0 & 0 & \Omega_\mathrm{ug} & 0 & 0 & \widetilde{E}_\mathrm{u}-\omega
\end{array}\right). \tag{S9}$$

Hereby, we use the abbreviation $\omega \equiv \omega_\beta(t)$, omit the time argument for all $\Omega$, mark gerade and ungerade state with a bar or a tilde, respectively, and separate blocks with a definite photon number $k$ by dashed lines. The two continuum energies are the same: $E = \overline{E}_\mathrm{g} = \widetilde{E}_\mathrm{u}$. Note the the couplings $\Omega_\mathrm{ug}$ between the two continuum state are much larger than among bound states ($\Omega_{01}$) or between bound and continuum states ($\Omega_{0\mathrm{g}}$ and $\Omega_{1\mathrm{u}}$). That is the reason that continuum states dressed by $\pm 1$ photons have to be included in the effective Hamilton matrix (S9).

In order to understand the emerging dynamics from matrix (S9), one should rearrange it by exchanging columns and rows to get

$$H_\mathrm{eff}(t) = \left(\begin{array}{cc|ccc|ccc}
\overline{E}_0+2\omega & \Omega_{01} & \Omega_{0\mathrm{u}} & 0 & 0 & 0 & 0 & 0 \\
\Omega_{10} & \widetilde{E}_1+\omega & 0 & \Omega_{1\mathrm{g}} & 0 & 0 & 0 & 0 \\ \hline
\Omega_{\mathrm{u}0} & 0 & \widetilde{E}_\mathrm{u}-\omega & \Omega_\mathrm{ug} & 0 & 0 & 0 & 0 \\
0 & \Omega_{\mathrm{g}1} & \Omega_\mathrm{gu} & \overline{E}_\mathrm{g} & \Omega_\mathrm{gu} & 0 & 0 & 0 \\
0 & 0 & 0 & \Omega_\mathrm{ug} & \widetilde{E}_\mathrm{u}+\omega & 0 & 0 & 0 \\ \hline
0 & 0 & 0 & 0 & 0 & \overline{E}_\mathrm{g}-\omega & \Omega_\mathrm{gu} & 0 \\
0 & 0 & 0 & 0 & 0 & \Omega_\mathrm{ug} & \widetilde{E}_\mathrm{u} & \Omega_\mathrm{ug} \\
0 & 0 & 0 & 0 & 0 & 0 & \Omega_\mathrm{gu} & \overline{E}_\mathrm{g}+\omega
\end{array}\right). \tag{S10}$$

Thereby we end up with three blocks: one consisting of bound states only and two decoupled blocks in the continuum. Only one of the two is connected to the bound-state block, the other one (at the bottom-right) is not and therefore can be neglected from now on.

In order to understand the chirp-dependent ionization dynamics we have to consider the four top-left blocks, which are given also in the text. In the diagonal, not only the 2×2 bound-state block, but also the 3×3 continuum-state block can be diagonalized analytically to get

$$H_{\text{eff}}(t) = \left(\begin{array}{cc:ccc:cccc} E_\downarrow & 0 & \cdot & C_\downarrow & \cdot & \cdot & \cdot & \cdot \\ 0 & E_\uparrow & \cdot & C_\uparrow & \cdot & \cdot & \cdot & \cdot \\ \hdashline \cdot & \cdot & \cdot & 0 & \cdot & \cdot & \cdot & \cdot \\ C_\downarrow & C_\uparrow & 0 & E & 0 & \cdot & \cdot & \cdot \\ \cdot & \cdot & \cdot & 0 & \cdot & \cdot & \cdot & \cdot \\ \hdashline \cdot & \cdot & \cdot & \cdot & \cdot & \cdot & \cdot & \cdot \\ \cdot & \cdot & \cdot & \cdot & \cdot & \cdot & \cdot & \cdot \\ \cdot & \cdot & \cdot & \cdot & \cdot & \cdot & \cdot & \cdot \end{array}\right), \tag{S11}$$

whereby matrix entries with a dot are not specified (they are not necessarily 0), since they are not relevant for the following discussion. The respective eigenvectors are

$$V_{\downarrow\uparrow} = \frac{1}{\sqrt{2}}\big(1, \pm 1\big) \qquad \text{and} \qquad \widetilde{V} = \frac{1}{\sqrt{2\Omega_{\text{ug}}{}^2 + \omega^2}}\big(-\Omega_{\text{ug}}, \omega, +\Omega_{\text{ug}}\big). \tag{S12}$$

Relevant are the two matrix elements connecting either of the adiabatic states with energy $E_{\downarrow\uparrow}$ with the continuum state at energy $E$. They read explicitly

$$C_{\downarrow\uparrow} = \frac{\mp\Omega_{0\text{u}}\Omega_{\text{ug}} - \omega\Omega_{1\text{g}}}{\sqrt{2\omega^2 + 4\Omega_{\text{ug}}{}^2}} \tag{S13}$$

and are given as Eq. (3) in the main text. Apparently, under the condition $\Omega_{0\text{u}}\Omega_{\text{ug}} = \omega\Omega_{1\text{g}}$ the two couplings $C_{\downarrow\uparrow}$ may have very different absolute values.

### 3.2 Strong-field propagated wavefunction

The Volkov propagator [see Eq. (5c) in the main text]

$$\hat{U}(t,t') = \mathrm{e}^{\mathrm{i}\int_{t'}^{t}\mathrm{d}t''[\hat{p}^2/2 + \hat{p}\,\mathcal{A}_\beta\cos(\omega_0 t'')]} \tag{S14}$$

is diagonal in the momentum representation

$$\big\langle k|\hat{U}(t,t')|k\big\rangle = \mathrm{e}^{\mathrm{i}\int_{t'}^{t}\mathrm{d}t''[k^2/2 + \mathcal{A}_\beta k\cos(\omega_0 t'')]} = \mathrm{e}^{\mathrm{i}[S(t) - k^2 t'/2 - \lambda\sin(\omega_0 t')]}, \tag{S15}$$

with $\lambda \equiv \mathcal{A}_\beta k/\omega_0$ being the electron-photon coupling parameter and $S(t) \equiv k^2 t/2 + \lambda\sin(\omega_0 t)$ accounting for a phase which is irrelevant for the absolute value of the amplitude (S15). By means of the Jacobi-Anger expansion the diagonal form of $\hat{U}$ reads

$$\big\langle k|U(t,t')|k\big\rangle = \mathrm{e}^{\mathrm{i}S(t)}\sum_{m=-\infty}^{+\infty}\mathrm{e}^{-\mathrm{i}[k^2/2 + m\omega_0]t'}J_m(\lambda). \tag{S16}$$

Inserting this into Eq. (5a) of the main text we get

$$\begin{aligned}\big\langle k|\psi(t\to\infty)\big\rangle = -\mathrm{i}\,\mathrm{e}^{\mathrm{i}S(t)}\lambda\omega_0 T_\beta\frac{\sqrt{\pi}}{2}\sum_m \mathrm{e}^{-\big[k^2/2 - [m+2]\omega_0 - E_0\big]^2 T_\beta{}^2} \\ \times\big[\text{sign}(\beta)J_{m+1}(\lambda)\langle k|0\rangle + J_m(\lambda)\langle k|1\rangle\big].\end{aligned} \tag{S17}$$

The dominant ionization channel is the two-photon absorption, collapsing the the sum in (S17) to the term $m = 0$, with the final continuum energy $k^2/2 = E_0 + 2\omega_0$ . Since the argument in the Bessel function is $\lambda \lesssim 1$, the term with $m = 0$ dominates. This allows for additionally retaining only the lowest order of $\lambda$ in the Bessel functions $J_0(\lambda) = 1 + \mathcal{O}(\lambda^2)$ and $J_1(\lambda) = \lambda/2 + \mathcal{O}(\lambda^3)$. Thus we may formulate the condition for ionization suppression as

$$\frac{\lambda}{2}\langle k|0\rangle = \langle k|1\rangle \qquad \text{or} \qquad \frac{\mathcal{A}_\beta}{2}\frac{\langle k|0\rangle}{\langle k|1\rangle} = \frac{\omega_0}{k}, \tag{S18}$$

where we have used in the latter version the explicit expression of the electron-photon coupling parameter $\lambda$, cf. its definition (6) in the main text. The condition for continuum suppression obtained from the dressed-state picture [Eq. (4) in the main text] and from the strong-field amplitude with a locked initial state [Eq. (S18) above] are equivalent. It can be shown that for large-$k$ continuum states $V_{\mathrm{ug}} = \frac{2}{\pi}k$ and $\sum_{j\in\mathrm{u}} V_{j\mathrm{g}} = k$, where the sum corresponds to the Volkov-propagated state.

## 4 Pulses "flipped" in time

We will proof that the final occupation of an initially populated state is the same in both cases, when the system is driven either by a pulse $F(t)$ or its "flipped" version $\widetilde{F}(t) \equiv F(-t)$. In other words the depletion of the initial state does not depend on the "direction" (i. e. in the cases studied in the text it does not depend on the sign of chirp) of the driving pulses.

Instead of looking at the TDSE (S3) it is convenient to consider the time-evolution operator $\hat{U}(t,t')$, which is also defined by a "TDSE", which reads in a basis or close-coupling representation

$$\mathrm{i}\frac{\partial}{\partial t}\boldsymbol{\mathcal{U}}(t,t') = \boldsymbol{\mathcal{H}}(t)\boldsymbol{\mathcal{U}}(t,t') \tag{S19}$$

with bold symbols denoting matrices and the Hamilton matrix in particular being $\boldsymbol{\mathcal{H}}(t) = H_{jj'}(t) = E_j\delta_{jj'} + F_\beta(t)\,V_{jj'}$ as in Eq. (S3). The formal solutions of (S19) read for both cases, i. e. driving by $F(t)$ and $\widetilde{F}(t)$, respectively,

$$\boldsymbol{\mathcal{U}}(+\tau,-\tau) = \mathrm{e}^{-\mathrm{i}\,\delta t\,\boldsymbol{\mathcal{H}}(t_n)}\ldots\mathrm{e}^{-\mathrm{i}\,\delta t\,\boldsymbol{\mathcal{H}}(t_1)}, \tag{S20a}$$

$$\widetilde{\boldsymbol{\mathcal{U}}}(+\tau,-\tau) = \mathrm{e}^{-\mathrm{i}\,\delta t\,\boldsymbol{\mathcal{H}}(t_1)}\ldots\mathrm{e}^{-\mathrm{i}\,\delta t\,\boldsymbol{\mathcal{H}}(t_n)}, \tag{S20b}$$

whereby we consider $n \to \infty$, $\delta t \to 0$, $n \times \delta t = 2\tau$, and $t_k = -\tau + [2k-1]\delta t$. By means of $\boldsymbol{\mathcal{H}}(t_k) = \boldsymbol{\mathcal{H}}^\top(t_k)$ one can deduce from the two sums (S20)

$$\widetilde{\boldsymbol{\mathcal{U}}}(+\tau,-\tau) = \boldsymbol{\mathcal{U}}^\top(+\tau,-\tau) \qquad \text{i. e.} \qquad \widetilde{\mathcal{U}}_{jj'}(+\tau,-\tau) = \mathcal{U}_{j'j}(+\tau,-\tau). \tag{S21}$$

In particular the special case $\widetilde{\mathcal{U}}_{jj}(+\tau,-\tau) = \mathcal{U}_{jj}(+\tau,-\tau)$ is interesting, since it guarantees that from $a_j(-\tau) = \widetilde{a}_j(-\tau) = \delta_{jj_{\mathrm{init}}}$ follows immediately $a_{j_{\mathrm{init}}}(+\tau) = \widetilde{a}_{j_{\mathrm{init}}}(+\tau)$ with $\tau$ being arbitrarily large. So indeed, the amplitudes of the initial state $j_{\mathrm{init}}$ are the same, irrespective of the "direction" of the pulse.

## References

[1] M. Wollenhaupt, A. Assion, and Th. Baumert, *Springer Handbook of Lasers and Optics*, chapter "Short and Ultrashort Laser Pulses", Springer Berlin Heidelberg (2012).

[2] N. V. Vitanov, T. Halfmann, B. W. Shore, and K. Bergmann, *Laser-induced population transfer by adiabatic passage techniques*. Annu. Rev. Phys. Chem. **52**, 763 (2001).

[3] X. M. Tong and C. D. Lin, *Empirical formula for static field ionization rates of atoms and molecules by lasers in the barrier-suppression regime*. J. Phys. B **38**, 2593 (2005).
